# Supplementary material for: Machine Learning of Accurate Energy-Conserving Molecular Force Fields
Source: arXiv:1611.04678 ancillary file (2017-05-08)
Supplement: Supplementary file 1 [file supplement.pdf]

# Machine Learning of Accurate Energy-Conserving Molecular Force Fields
Supplement

Stefan Chmiela,[1] Alexandre Tkatchenko,[2,3,*] Huziel Sauceda,[3]
Igor Poltavsky,[2] Kristof T. Schütt,[1] and Klaus-Robert Müller[1,4,†]

[1]*Machine Learning Group, Technische Universität Berlin, 10587 Berlin, Germany*
[2]*Physics and Materials Science Research Unit, University of Luxembourg, L-1511 Luxembourg*
[3]*Fritz-Haber-Institut der Max-Planck-Gesellschaft, 14195 Berlin, Germany*
[4]*Department of Brain and Cognitive Engineering,*
*Korea University, Anam-dong, Seongbuk-gu, Seoul 136-713, Korea*
(Dated: May 8, 2017)

## S1. NOISE AMPLIFICATION BY DIFFERENTIATION

When estimating interatomic forces from a statistical model trained on energies, considerable noise will likely be present. This is because the derivative operator amplifies high frequencies with increasing gain, which – per assumption – is the frequency band noise lives in: the derivative of a model $f$ in the frequency domain is

$$\mathcal{F}\left[f'\right] = \mathrm{i}\omega\mathcal{F}\left[f\right], \tag{1}$$

with $\mathcal{F}[f]$ being its Fourier transform.

As functions parameterized by data are inherently noisy, either because the data itself is imprecise or due to the ill-posedness of the model, this phenomenon can not be avoided. Commonly, machine learning approaches alleviate noise effects via regularization, i.e. by attenuating parts of the model's frequency spectrum that are assumed to be distorted [31]. Model de-noising can also be implemented as a post-processing step by recovering low-dimensional data manifolds from high-dimensional embeddings for example by means of principal component analysis (PCA) [32–35]. In most cases however, the resulting predictor will never exactly match the truth so that the differentiation process will still amplify the remaining noise and increase the prediction error.

## S2. VECTOR-VALUED KERNEL LEARNING

The predictor used in this work is a generalization of the commonly used kernel ridge-regression technique to structured vector fields [19–21]. Like its scalar counterpart, it transforms the input to a high-dimensional feature space $\phi\colon \mathcal{X} \to \mathcal{H}$ where the data can be modeled by a linear function. Adopting the kernel trick [36], this space is defined implicitly through a kernel function $\kappa(\vec{x}, \vec{x}') = \langle \phi(\vec{x}), \phi(\vec{x}') \rangle_{\mathcal{H}}$ that characterizes the inner product in some reproducing kernel Hilbert space $\mathcal{H}$.

* alexandre.tkatchenko@uni.lu
† klaus-robert.mueller@tu-berlin.de

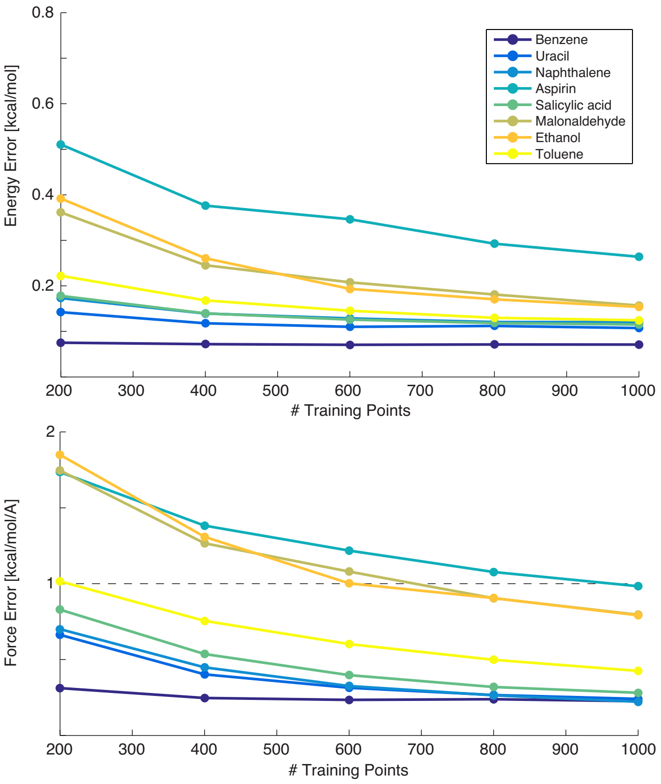


FIG. S1. The accuracy of the GDML model (in terms of the mean absolute error) as a function of training set size: chemical accuracy of less than 1 kcal mol$^{-1}$ is already achieved for small training sets.

Kernels replace the covariance term in the normal equation of the ridge estimator. GDML solves the derivative of this normal equation and maps to all partial forces of a molecule simultaneously. Rearranging the kernel term $\kappa\left(\frac{\partial x_i}{\partial \mathbf{R}}, \frac{\partial x'}{\partial \mathbf{R}}\right) = \frac{\partial^2 \kappa}{\partial^2 \mathbf{R}}$ reveals that the force-field kernel is the Hessian matrix of any kernel function that is at least twice differentiable. The efficient use of samples and the convex nature of the GDML optimization problem enables us to train the model using a direct solver with all its numerical benefits. The regularization coefficient $\lambda$ as well as the length scale $\sigma$ and the smoothness parameter $v$ of the Matérn kernel are found through a grid

TABLE S1. Properties of MD datasets that were used for numerical testing. Forces are in kcal mol$^{-1}$ Å$^{-1}$, energies in kcal mol$^{-1}$.

| Dataset | | | | Energies | | | Forces | | |
|---|---|---|---|---|---|---|---|---|---|
| Molecule | Formula | DOF | Size | Range | Min. ($\times 10^4$) | Max. ($\times 10^4$) | Range | Min. | Max. |
| Benzene | $C_6H_6$ | 30 | 627000 | 20.2 | −14.653 | −14.651 | 266.3 | −126.677 | 139.626 |
| Uracil | $C_4H_4N_2O_2$ | 30 | 133000 | 39.9 | −26.012 | −26.008 | 476.6 | −237.381 | 239.249 |
| Naphthalene | $C_{10}H_8$ | 48 | 326000 | 48.4 | −24.192 | −24.187 | 452.9 | −217.207 | 235.688 |
| Aspirin | $C_9H_8O_4$ | 57 | 211000 | 47.0 | −40.676 | −40.671 | 404.1 | −195.664 | 208.454 |
| Salicylic acid | $C_7H_6O_3$ | 42 | 320000 | 47.5 | −31.105 | −31.100 | 453.8 | −236.086 | 217.687 |
| Malonaldehyde | $C_3H_4O_2$ | 21 | 993000 | 43.8 | −16.751 | −16.747 | 570.7 | −286.050 | 284.602 |
| Ethanol | $C_2H_6O$ | 21 | 555000 | 35.5 | −9.721 | −9.717 | 432.0 | −211.104 | 220.900 |
| Toluene | $C_7H_8$ | 39 | 442000 | 46.9 | −17.024 | −17.019 | 425.6 | −212.984 | 212.617 |

TABLE S2. GDML prediction accuracy for interatomic forces and total energies for all datasets. Energy errors are in kcal mol$^{-1}$, force errors in kcal mol$^{-1}$ Å$^{-1}$.

| Dataset | | Energy Prediction | | Force Prediction | | | | | |
|---|---|---|---|---|---|---|---|---|---|
| | | | | | | Magnitude | | Angle | |
| Molecule | # ref. | MAE | RMSE | MAE | RMSE | MAE | RMSE | MAE | RMSE |
| Benzene | 1000 | 0.07 | 0.09 | 0.23 | 0.34 | 0.21 | 0.30 | 0.0041 | 0.0079 |
| Uracil | 1000 | 0.11 | 0.14 | 0.24 | 0.38 | 0.24 | 0.33 | 0.0040 | 0.0066 |
| Naphthalene | 1000 | 0.12 | 0.15 | 0.23 | 0.34 | 0.21 | 0.28 | 0.0033 | 0.0115 |
| Aspirin | 1000 | 0.27 | 0.36 | 0.99 | 1.41 | 0.91 | 1.19 | 0.0169 | 0.0244 |
| Salicylic acid | 1000 | 0.12 | 0.15 | 0.28 | 0.43 | 0.32 | 0.43 | 0.0038 | 0.0065 |
| Malonaldehyde | 1000 | 0.16 | 0.25 | 0.80 | 1.15 | 0.71 | 0.97 | 0.0109 | 0.0184 |
| Ethanol | 1000 | 0.15 | 0.20 | 0.79 | 1.12 | 0.99 | 1.33 | 0.0130 | 0.0237 |
| Toluene | 1000 | 0.12 | 0.16 | 0.43 | 0.62 | 0.35 | 0.45 | 0.0055 | 0.0088 |

search of a suitable subset of the hyper-parameter space. Throughout, cross-validation with dedicated datasets for training and testing is used to estimate the generalization performance of the model. Finally, the model is evaluated on a separate, previously unseen hold-out set (see e.g. Hansen et al. [13]).

## S3. DESCRIPTORS

We use an input descriptor $D$ to disambiguate Cartesian geometries that are physically equivalent. Inspired by the Coulomb matrix [11], geometries are represented by matrices were each entry

$$D_{ij} = \begin{cases} \|R_i - R_j\|^{-1} & \text{for } i > j \\ 0 & \text{for } i \leq j \end{cases} \quad (2)$$

is the reciprocal of the Euclidian distance of two atoms. When used with a descriptor, the covariance structure defined by the kernel must be projected back from descriptor space $\mathcal{D}$ to the original input space $\mathcal{I}$ to match the Cartesian force labels. The result $\kappa_{\mathcal{D}\to\mathcal{I}} = \partial\mathbf{D}^\top \kappa \partial\mathbf{D}'$ is given by the chain rule were $\partial\mathbf{D} = (\partial D_1/\partial\mathbf{R}, \ldots, \partial D_N/\partial\mathbf{R})$ is the matrix of partial derivatives of the (vectorized) training descriptors in each column.

## S4. MODEL ANALYSIS

We analyze the performance of all models using the well established mean absolute error (MAE) and root-mean-square error (RMSE) measures for both, energy and force predictions (see Tables S4 and S2 and Fig. S1). Since forces are multivariate, we analyze them under two additional aspects that permit a better assessment of their topological accuracy: The magnitude error $\|\hat{f}\| - \|f\|$ describes the extend to which the slope of the predicted PES differs from the reference calculation. We measure MAE and RMSE of the magnitudes of predicted and true forces. The angular error $\cos^{-1}(\hat{f}/\|\hat{f}\| \cdot f/\|f\|)/\pi$ measures the relative orientation of the predicted force direction and the reference. An error of zero indicates perfect alignment, while an error of one shows that the predicted vector is inverted. Again, we compute the MAE and the RMSE of this quantity. Fig. S2 shows qualitatively, how closely the predicted energies and forces follow the reference data (using the ex-

TABLE S3. Accuracy of the naïve force predictor. This model learns all components of the force labels independently. It is identical to the GDML model in all aspects, except for being energy-conservative. Energy errors are in kcal $mol^{-1}$, force errors in kcal $mol^{-1}$ $Å^{-1}$.

| Dataset | | Energy Prediction | | Force Prediction | | | | | |
|---|---|---|---|---|---|---|---|---|---|
| | | | | | | Magnitude | | Angle | |
| Molecule | # ref. | MAE | RMSE | MAE | RMSE | MAE | RMSE | MAE | RMSE |
| Benzene | 1000 | n/a | n/a | 14.67 | 20.01 | 19.38 | 22.39 | 0.4496 | 0.5048 |
| Uracil | 1000 | n/a | n/a | 5.91 | 11.29 | 1.90 | 2.84 | 0.1341 | 0.1859 |
| Naphthalene | 1000 | n/a | n/a | 6.50 | 11.16 | 2.17 | 3.13 | 0.1255 | 0.1748 |
| Aspirin | 1000 | n/a | n/a | 8.80 | 12.95 | 6.64 | 9.29 | 0.1481 | 0.1948 |
| Salicylic acid | 1000 | n/a | n/a | 6.13 | 11.28 | 2.36 | 3.35 | 0.1183 | 0.1662 |
| Malonaldehyde | 1000 | n/a | n/a | 19.98 | 27.35 | 17.99 | 22.79 | 0.4157 | 0.4664 |
| Ethanol | 1000 | n/a | n/a | 18.15 | 24.78 | 24.12 | 30.89 | 0.3938 | 0.4506 |
| Toluene | 1000 | n/a | n/a | 15.66 | 23.29 | 11.85 | 16.09 | 0.3583 | 0.4109 |

TABLE S4. Accuracy of the converged energy-based predictor. All training set sizes are chosen to match the complexity of the optimization problem in the corresponding force model (number of samples times number of partial derivatives). Energy errors are in kcal $mol^{-1}$, force errors in kcal $mol^{-1}$ $Å^{-1}$.

| Dataset | | Energy Prediction | | Force Prediction | | | | | |
|---|---|---|---|---|---|---|---|---|---|
| | | | | | | Magnitude | | Angle | |
| Molecule | # ref. | MAE | RMSE | MAE | RMSE | MAE | RMSE | MAE | RMSE |
| Benzene | 36000 | 0.04 | 0.06 | 0.80 | 1.16 | 1.00 | 1.38 | 0.0196 | 0.0350 |
| Uracil | 36000 | 0.03 | 0.03 | 0.44 | 0.62 | 0.45 | 0.54 | 0.0092 | 0.0148 |
| Naphthalene | 54000 | 0.02 | 0.03 | 0.40 | 0.55 | 0.43 | 0.52 | 0.0079 | 0.0129 |
| Aspirin | 63000 | 0.03 | 0.04 | 1.51 | 2.12 | 0.98 | 1.28 | 0.0220 | 0.0311 |
| Salicylic acid | 48000 | 0.10 | 0.13 | 0.45 | 0.63 | 0.39 | 0.51 | 0.0052 | 0.0090 |
| Malonaldehyde | 27000 | 0.11 | 0.16 | 0.83 | 1.16 | 0.80 | 1.05 | 0.0128 | 0.0230 |
| Ethanol | 27000 | 0.09 | 0.14 | 0.76 | 1.07 | 0.92 | 1.22 | 0.0116 | 0.0246 |
| Toluene | 45000 | 0.06 | 0.08 | 0.52 | 0.71 | 0.50 | 0.61 | 0.0087 | 0.0146 |

ample of uracil).

## S5. DETAILS OF THE PIMD SIMULATION

Path-integral molecular dynamics (PIMD) is a method that incorporates quantum-mechanical effects into molecular dynamics simulations using Feynman's path integral formalism. Here, PIMD simulations were done using $P = 10$ beads at ambient temperature using the GDML model implemented in the i-PI code [30]. The recently developed estimators based on perturbation theory were used to evaluate structural and electronic observables [29]. The total time of simulation was 200 ps for aspirin and 100 ps for the rest of the molecules, and for all the cases the NVT ensemble was used with a time step of 0.5 fs.

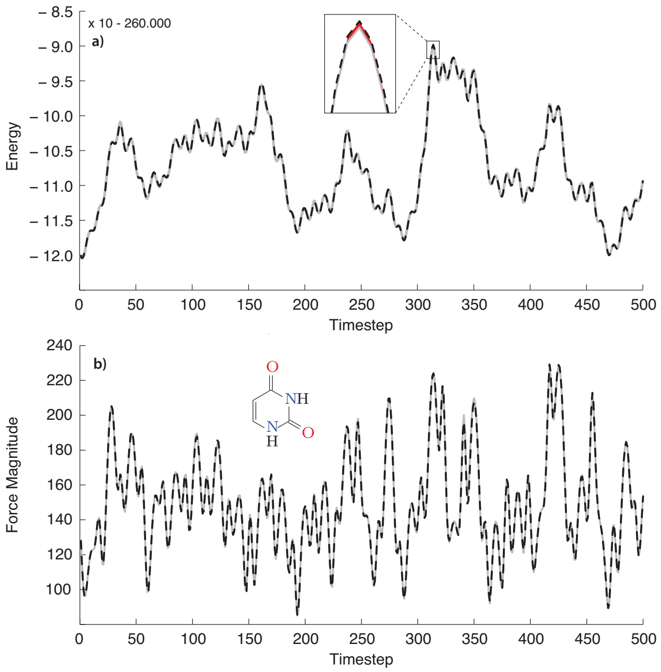


FIG. S2. Predicting energies (a) and forces (b) for 500 consecutive time steps of an MD simulation of uracil at 500 K. The prediction (gray) follows the reference trajectory (black, dashed) with high accuracy. The area between both curves is marked red to highlight small deviations.
